# Supplementary material for: On Train-Test Class Overlap and Detection for Image Retrieval
Source: arXiv:2404.01524 source file (2024-04-01)
Supplement: Supplementary file 2 [file supp-2.tex]

\clearpage

\title{Supplementary material for \\ ``On Train-Test Class Overlap and Detection for Image Retrieval''}
%\author{}

\maketitle
\thispagestyle{empty}

% PAGE NUMBER SET TO 1
 \setcounter{page}{1}

% LINE NUMBER SET TO 1
%\cvprulercount=1

% START APPENDIX
\appendix

% NUMBERING

%------------------------------------------------------------------------------

\section{Implementation Details}
\label{sec:Implementation}

In our experimental setup, we utilize a computational environment featuring 8 RTX 3090 GPUs and deploy PyTorch\cite{Paszke01} for all implementations. We leverage transfer learning, utilizing pre-trained ImageNet\cite{Russakovsky01} models as a foundational layer for training. To ensure a fair comparison with previous studies \cite{yang2021dolg, SCH01, tokens}, we configure the learning environment as closely as possible to the earlier benchmarks. Specifically, we employ ResNet101~\cite{Zhang01} as the backbone architecture and set the final feature dimension to 2048.

ArcFace loss\cite{Deng01} is the chosen loss function for training, with a margin parameter set at 0.3. Stochastic gradient descent is used for optimization, featuring a momentum of 0.9 and a weight decay rate of 0.00001. The initial learning rate is set at 0.001, and we include a warm-up phase~\cite{He2018BagOT} spanning three epochs.
Previous research has shown the effectiveness of preserving the original image resolution during the training of image search models~\cite{Hao2016WhatIT, Gordo01}. We adopt this principle and apply methods\cite{Yokoo01, SCH01, dtop}, where each training batch consists of images with similar aspect ratios instead of a single fixed size. The batch size for training is set at 128. Following the methodologies in DIR~\cite{Gordo01} and DELF~\cite{delf} studies, we carry out classification-based training on the initial dataset and subsequently fine-tune the model. During this fine-tuning stage, the layers of the Resnet101 backbone are frozen (\autoref{fig:A5_FT}).

For evaluation purposes, we employ multi-resolution representation~\cite{Gordo01} on both query and database images and apply $\ell_2$-normalization and whitening techniques~\cite{Radenovic01} on the final feature.

%------------------------------------------------------------------------------

\section{Benchmark}
\label{sec:Benchmark}

\begin{figure*}
\centering
% \fig[1.0]{2}
\scriptsize
\setlength{\tabcolsep}{4pt}
\begin{tabular}{cc}
\fig[.5]{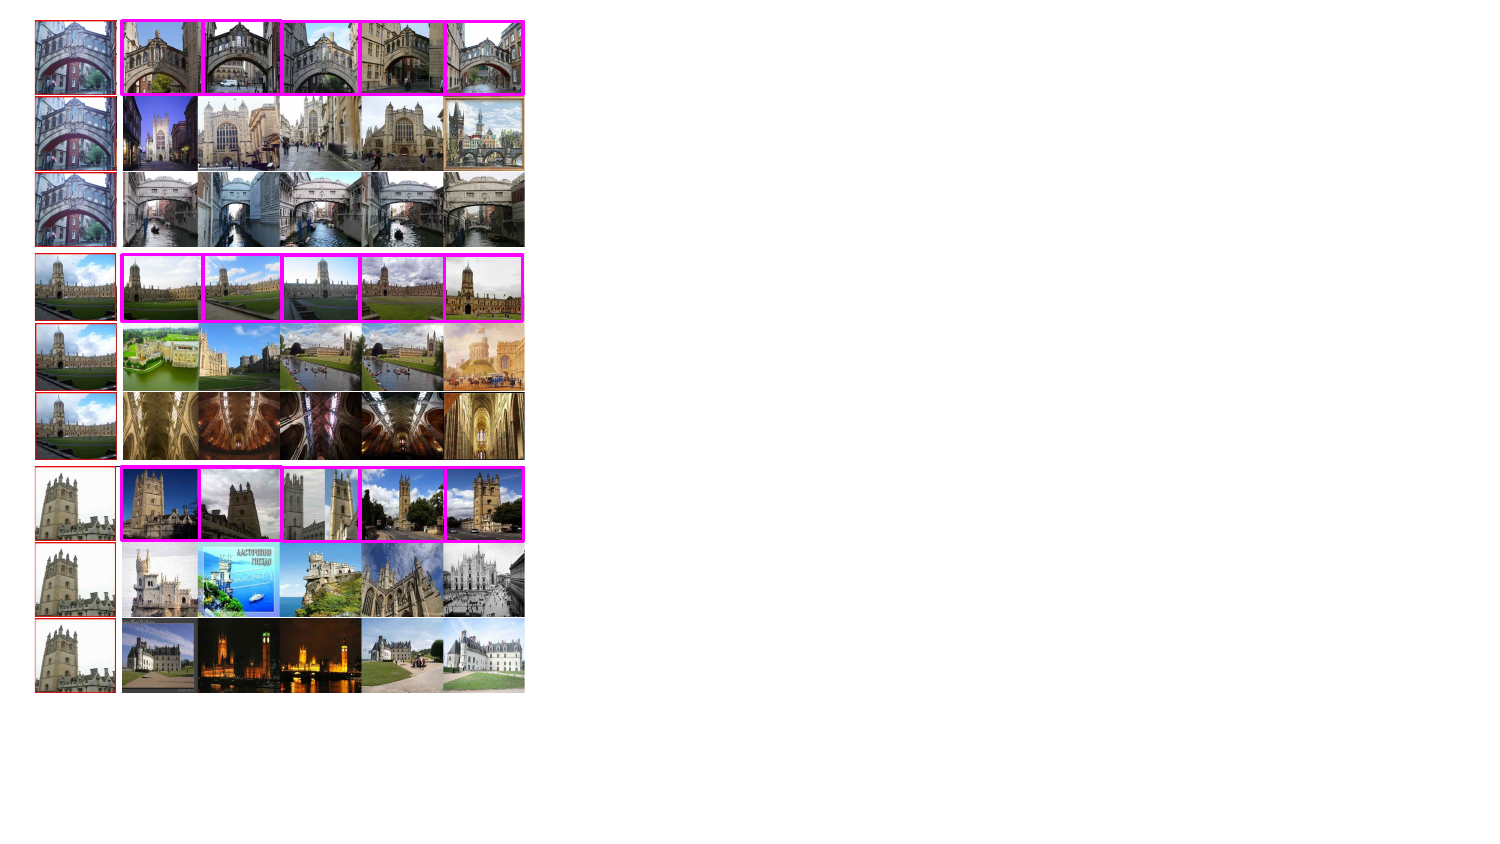} & \fig[.5]{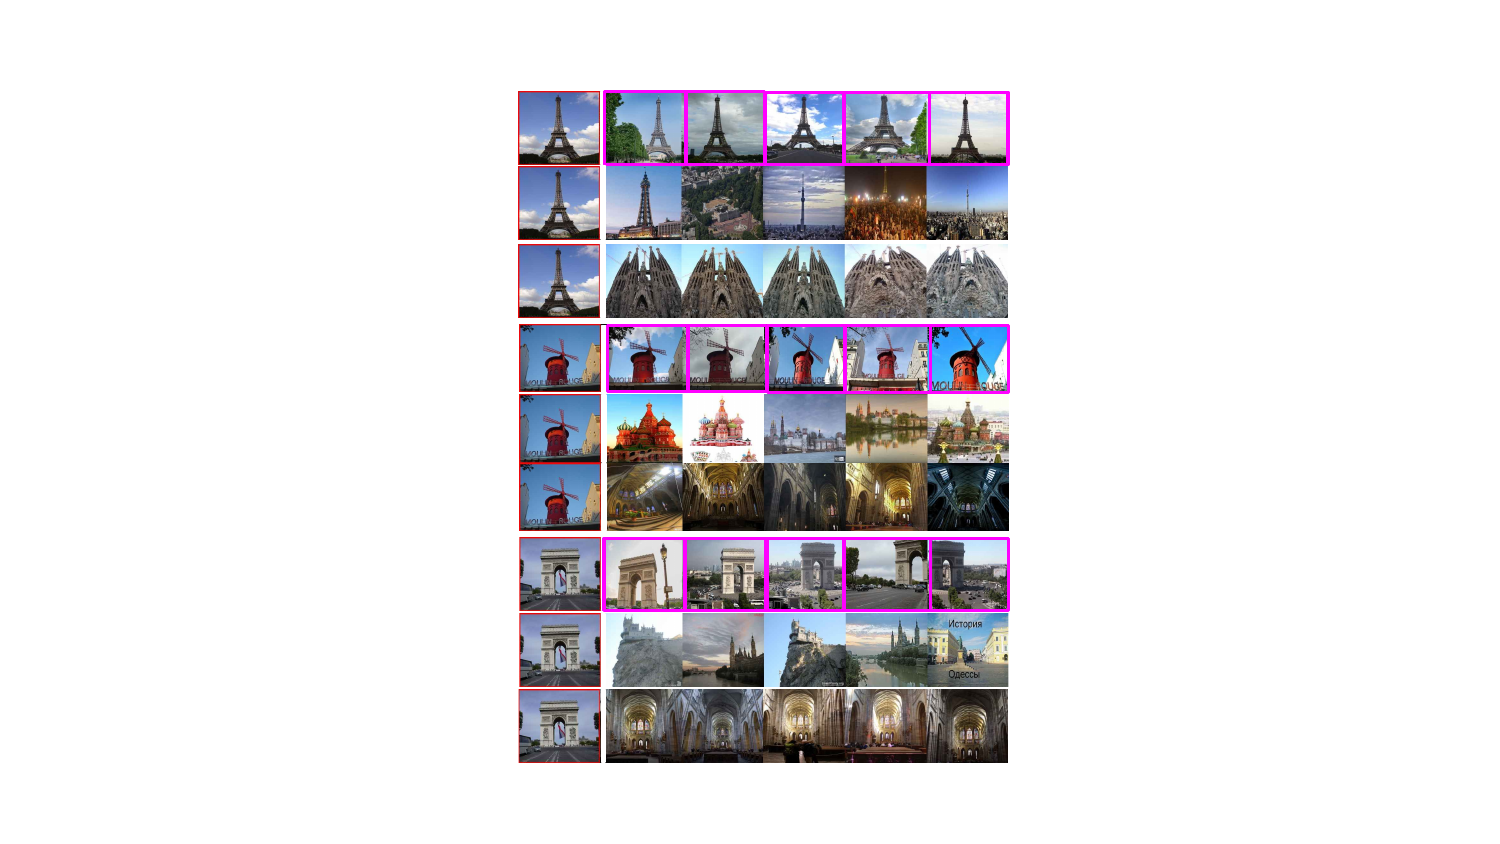} \\[3pt]

Evaluation: $\cR$Oxford & Evaluation: $\cR$Paris \\
\end{tabular}
\vspace{-6pt}
\caption{\emph{Confirming overlapping landmark categories} between training sets (GLDv2-clean, NC-clean, SfM-120k) and evaluation sets ($\cR$Oxford, $\cR$Paris). Red box: query image. The query image from the evaluation set in each box/row is followed by top-5 most similar images from the training set. Pink box: training image landmark identical with query (evaluation) image landmark.
}
\label{fig:fig2_sup}
\end{figure*}
%------------------------------------------------------------------------------

\autoref{tab:param} shows the model complexity\footnote{\url{https://github.com/sovrasov/flops-counter.pytorch}} results for a single forward pass for each model, given an input image of size 224 $\times$ 224.
R101 in this table is the baseline for all related studies, as it basically only uses the last feature map layer.
In this table, we can see that our study uses the fewest parameters and computational complexity, after Yokoo~\etal~\cite{Yokoo01}, which only uses GeM+FC. Note that the model complexity results in this table were only tested on the studies that provided official code. And, \autoref{tab:param2} shows the results of the model complexity for each of the components mentioned in \autoref{sec:impl}.

%------------------------------------------------------------------------------
\begin{table}
\centering
\scriptsize
\setlength{\tabcolsep}{5.5pt}
\begin{tabular}{lcc} \toprule
\Th{Network} & \Th{\#Params (M)} & \Th{\#GFLOPs} \\ \midrule
R101 & 42.50 & 7.86 \\
Yokoo~\etal~\cite{Yokoo01} & 43.91 & 7.86  \\
SOLAR~\cite{Ng01} & 53.36 & 8.57 \\
DOLG~\cite{yang2021dolg} & 47.07 & 8.07 \\
Token~\cite{tokens} & 54.43 & 8.05 \\
CiDeR (Ours) &  46.12 & 7.94 \\
\bottomrule
\end{tabular}
\vspace{-6pt}
\caption{ \emph{Parameter} (\Th{\#Params}) and  \emph{Computational Complexity} comparison (\Th{\#GFLOPs}) between ours \vs previous studies.}
\label{tab:param}
\end{table}
%------------------------------------------------------------------------------

%------------------------------------------------------------------------------
\begin{table}
\centering
\scriptsize
\setlength{\tabcolsep}{3.0pt}
\begin{tabular}{ccccccc} \toprule
\Th{R101} & \Th{BE} & \Th{SC} & \Th{AL} &\Th{ Pooling} & \Th{\#Params (M)} & \Th{\#GFLOPs} \\ \midrule
\ch &     &      &     &  & 42.50 & 7.86  \\
\ch & \ch &      &     &  & 43.58 & 7.91 \\
\ch & \ch & \ch  &     &  & 43.88 & 7.93 \\
\ch & \ch & \ch  & \ch &  & 44.02 & 7.94 \\
\ch & \ch & \ch  & \ch & \ch & 46.12 & 7.94 \\
\bottomrule
\end{tabular}
\vspace{-3pt}
\caption{ \emph{Parameter} (\Th{\#Params}) and  \emph{Computational Complexity} comparison (\Th{\#GFLOPs}) between ours each components. BE: backbone enhancement; SC: selective context; AL: attentional localization; Pooling:Spaital Pooling(GeM)+FC.
}
\label{tab:param2}
\end{table}
%------------------------------------------------------------------------------

\section{More on revisiting Google Landmarks v2}

%------------------------------------------------------------------------------
\begin{table*}
\centering
\scriptsize
\begin{tabular}{cccll} \toprule
\Th{\#} & \Th{GID} & \Th{\# Images} & \Th{GLDv2 Landmark Name} & \Th{Oxford/Paris Landmark Name} \\
\midrule
 1 &   6190 & 98 & \href{http://commons.wikimedia.org/wiki/Category:Radcliffe_Camera}{Radcliffe Camera} & Oxford \\
 2 &  19172 & 32 & \href{http://commons.wikimedia.org/wiki/Category:All_Souls_College,_Oxford}{All Souls College, Oxford} & All Souls Oxford\\
 3 &  37135 & 18  & \href{http://commons.wikimedia.org/wiki/Category:Oxford_University_Museum_of_Natural_History}{Oxford University Museum of Natural History} & Pitt Rivers Oxford \\
 4 &  42489 & 55 & \href{http://commons.wikimedia.org/wiki/Category:Pont_au_Double}{Pont au Double} & Jesus Oxford\\
5 & 147275 & 18 & \href{http://commons.wikimedia.org/wiki/Category:Magdalen_Tower}{Magdalen Tower} & Ashmolean Oxford \\
6 & 152496 & 71 & \href{http://commons.wikimedia.org/wiki/Category:Christ_Church,_Oxford}{Christ Church, Oxford} & Christ Church Oxford\\
7 & 167275 & 55 & \href{http://commons.wikimedia.org/wiki/Category:Bridge_of_Sighs_(Oxford)}{Bridge of Sighs (Oxford)} & Magdalen Oxford \\
8 & 181291 & 60 & \href{http://commons.wikimedia.org/wiki/Category:Petit-Pont}{Petit-Pont} & Notre Dame Paris \\
9 & 192090 & 23 & \href{http://commons.wikimedia.org/wiki/Category:Christ_Church_Great_Quadrangle}{Christ Church Great Quadrangle} & Paris  \\
10 &  28949 & 91 & \href{http://commons.wikimedia.org/wiki/Category:Moulin_Rouge}{Moulin Rouge} & Moulin Rouge Paris \\
11 &  44923 & 41 & \href{http://commons.wikimedia.org/wiki/Category:Jardin_de_l'Intendant}{Jardin de l'Intendant} & Hotel des Invalides Paris \\
12 &  47378 & 731  & \href{http://commons.wikimedia.org/wiki/Category:Eiffel_Tower}{Eiffel Tower} & Eiffel Tower Paris \\ % 731+(23+150%%%추)
13 &  69195 & 34 & \href{http://commons.wikimedia.org/wiki/Category:Place_Charles-de-Gaulle_(Paris)}{Place Charles-de-Gaulle (Paris)} & Arc de Triomphe Paris \\ %%%%추 22 > 150-177
14 & 167104 & 23 & \href{http://commons.wikimedia.org/wiki/Category:H%C3%B4tel_des_Invalides}{Hôtel des Invalides} & Hotel des Invalides Paris \\
15	& 145268 & 72 & \href{http://commons.wikimedia.org/wiki/Category:Louvre_Pyramid}{Louvre Pyramid} & Louvre Paris\\
16	& 146388 & 80 & \href{http://commons.wikimedia.org/wiki/Category:Basilique_du_Sacr%C3%A9-C%C5%93ur_de_Montmartre}{Basilique du Sacré-Cœur de Montmartre} & Arc de Triomphe Paris  \\
17 & 138332 & 30 & \href{http://commons.wikimedia.org/wiki/Category:Parvis_Notre-Dame_-_place_Jean-Paul-II_(Paris)}{Parvis Notre-Dame - place Jean-Paul-II (Paris)} & Notre Dame Paris  \\
18 & 144472 & 33 & \href{http://commons.wikimedia.org/wiki/Category:Esplanade_des_Invalides}{Esplanade des Invalides} & Paris \\
\bottomrule
\end{tabular}
\vspace{-6pt}
\caption{GIDs information removed in GLDv2-clean dataset. % $\cR$GLDv2-clean:
\iavr{Please add columns with landmark names of both GLD and Ox/Par, one more column with overlapped dataset (Ox or Par) and one with the number of images in each GID, as indicated. }}
\label{tab:removing_gid}
\end{table*}

We employ GLAM~\cite{SCH01} to extract image features from the training and evaluation sets. Extracted features from the training sets are indexed using the Approximate Nearest Neighbor (ANN)\footnote{\url{https://github.com/kakao/n2}} search method. For verification, we use SIFT~\cite{Lowe01} local descriptors. We find tentative correspondences between local descriptors by a kd-tree and we verify by obtaining inlier correspondences using RANSAC.

\autoref{fig:fig2_sup} shows another set of additional results to \autoref{fig:fig2} in~\autoref{sec:dataset}.
In the figure, we can also see the overlapping landmark categories between the training set (GLDv2-clean, NC-clean, SfM-120k) and the evaluation set ($\cR$Oxford, $\cR$Paris).
In other words, only GLDv2-clean has overlapping results with the evaluation set.

Using the method described above, we determine the final GID.
~\autoref{tab:removing_gid} shows the details of the 18 GIDs that are cleared due to overlapping in GLDv2-Clean mentioned in~\autoref{tab:table1}.
Then, by removing the images belonging to the GIDs in this table, we open the new $\cR$GLDv2-clean dataset.

%------------------------------------------------------------------------------

\section{More ablations}
\label{sec:mAblation}

%------------------------------------------------------------------------------
\begin{figure*}[t]
\begin{center}
	\fig[1.0]{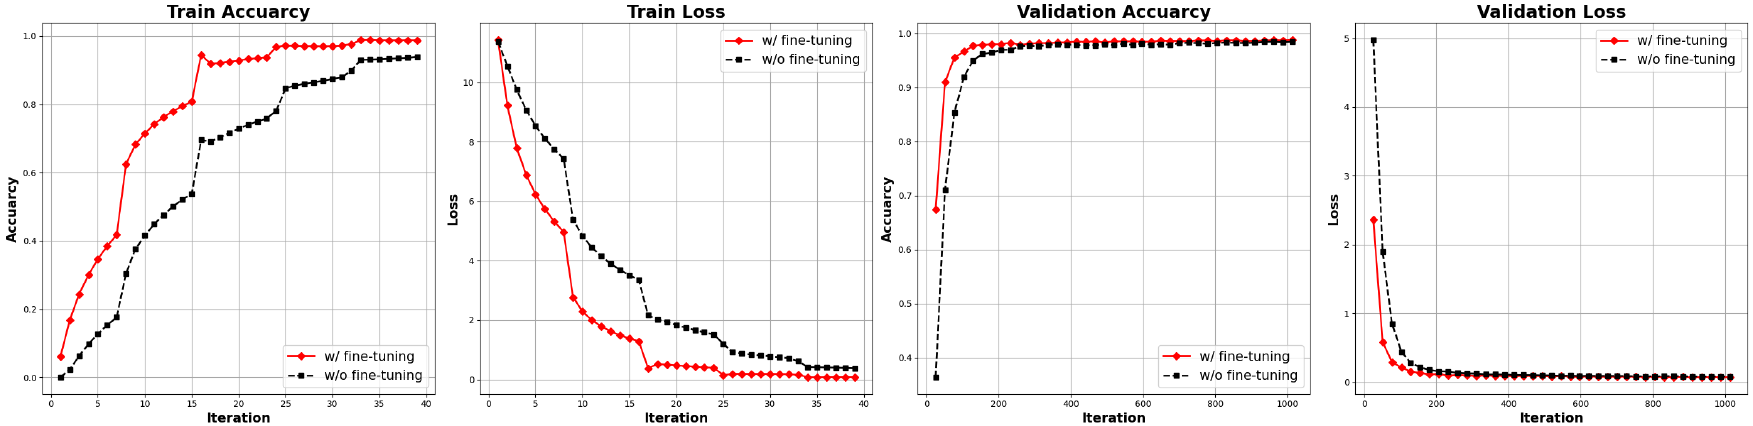}
\end{center}
\vspace{-12pt}
\caption{Comparison of the accuracy/loss for training and validation of models \emph{with (red) \vs without (black) Fine-tuning}.}
\label{fig:ft}
\end{figure*}
%------------------------------------------------------------------------------

%------------------------------------------------------------------------------
\begin{figure}[t]
\centering
\fig[.9]{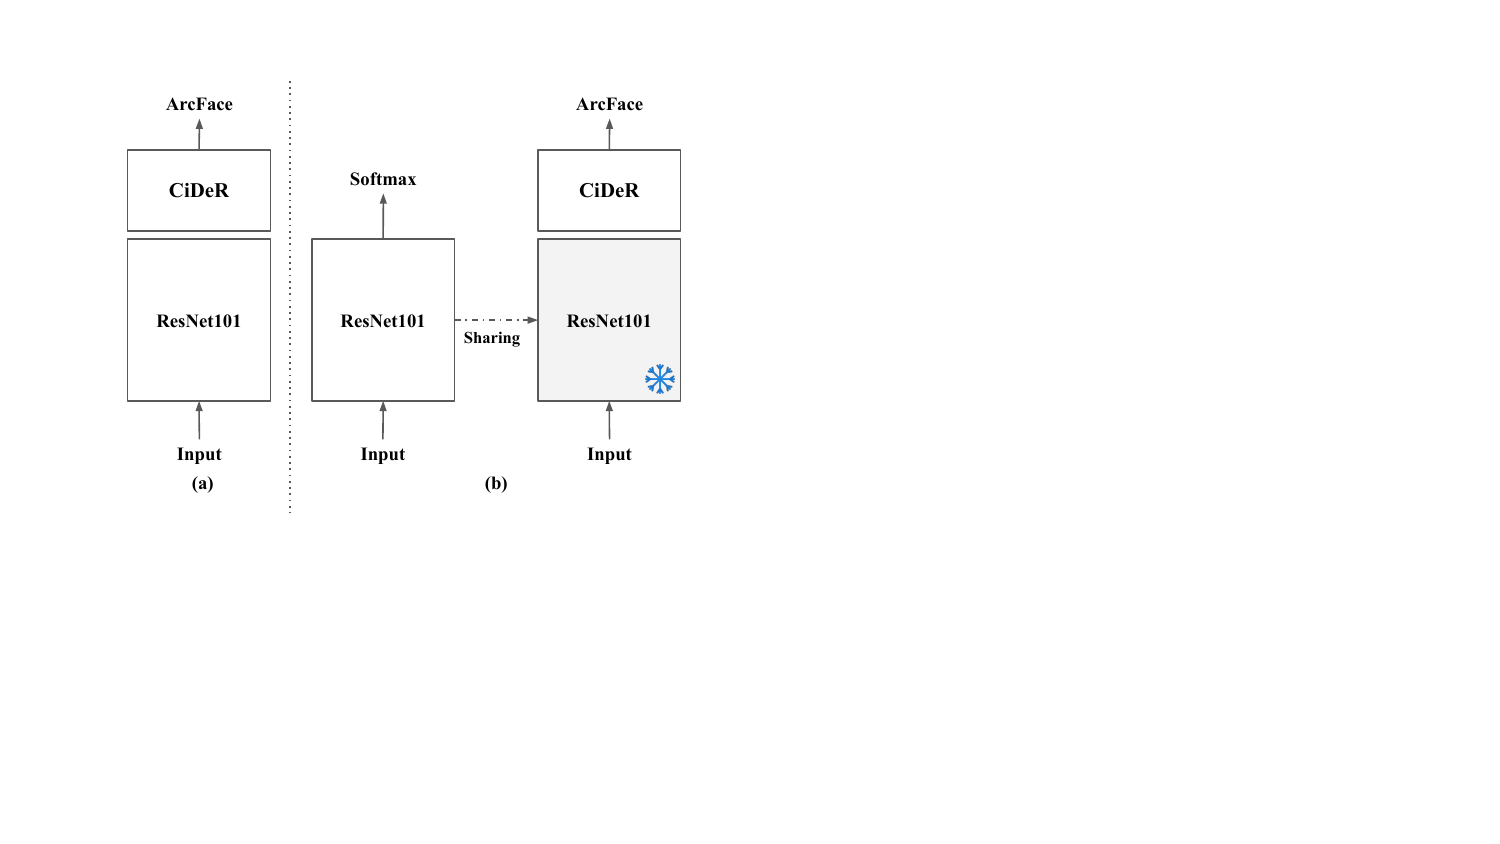}
\caption{Our fine-tuning procedures. (a) None fine-tuning. (b) Ours fine-tuning. \includegraphics[height=0.3cm]{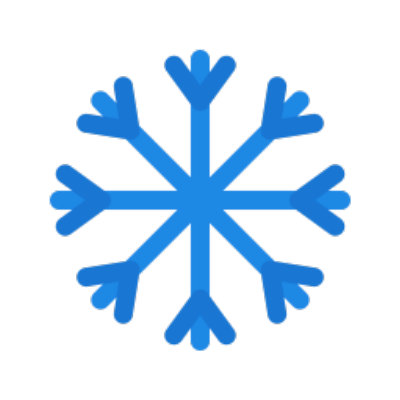}:frozen.}
\vspace{-12pt}
\label{fig:A5_FT}
\end{figure}
%------------------------------------------------------------------------------

\paragraph{Fine-tuning}

We generally employ a fine-tuning method, utilizing models pre-trained on ImageNet. Following the methods of DIR~\cite{Gordo01} and DELF~\cite{delf},
%we conduct classification-based training first, then fine-tune our model to achieve significant performance improvements.
we achieve significant performance gains by performing classification-based training with a landmark trainset and then fine-tuning the model with the same trainset again.
In particular, we freeze the ResNet101 backbone layers and only train the network proposed in \autoref{sec:1-stage}. \autoref{fig:A5_FT} visualizes this process, while \autoref{fig:ft} shows the training and validation loss and accuracy.
These graphs affirm that fine-tuning ($\mathbf{w/ \, fine}$-$\mathbf{tuning}$) results in lower loss and higher accuracy across both training and validation sets.
This is corroborated by improved performance results ({\ours+FT}) in \autoref{tab:1m}.
Compared to the results without the fine-tuning, we note gains of 2.7\% and 3.1\% on \oxf5k and \paris6k Base, 8.9\% and 5.1\% on \rox and \rpa Medium, and 16.5\% and 11.4\% on \rox and \rpa Hard.

%------------------------------------------------------------------------------

\paragraph{Backbone Enhancement (BE)}

In this experiment, we apply four methods that can be utilized in a plug-and-play fashion~\cite{wang01, Wang02, GatherExcite, Hu01}. ~\autoref{tab:senet} shows the results of the experiment. SENet~\cite{Hu01} is selected as it showed the best performance in the experiment.
% \autoref{sec:1-stage}에서 설명한 EBM에 대한 실험 결과이다.
% 이 실험에서  plug in play 방식으로 활용할 수 있는 4가지 방법을 적용한다.
% ~\autoref{tab:senet}에서 실험 결과를 보여준다.
% 이 실험결과에서, SENet~\cite{Hu01}이 가장 좋은 성능을 보였고 우리는 이를 선택한다.

%------------------------------------------------------------------------------
\begin{table}[t]
\centering
\scriptsize
%\tiny
\setlength{\tabcolsep}{5.0pt}
\begin{tabular}{l*{7}{c}} \toprule
\mr{2}{\Th{Method}} & \mr{2}{\Th{Oxf5k}} & \mr{2}{\Th{Par6k}} & \mc{2}{\Th{Medium}} & \mc{2}{\Th{Hard}} \\ \cmidrule(l){4-7}
 & & &  \rox & \rpa & \rox & \rpa \\ \midrule
ECNet~\cite{wang01} &  88.2     & {91.5} & {66.8}      & {78.3}       & {42.0}       & {55.4}       \\
NLNet~\cite{Wang02}           & 89.4      & {91.8} &  {66.5}     & {77.6}      & {39.1}       & {53.7}  \\
Gather-Excite~\cite{GatherExcite} &  89.4     & {90.5} &  {66.7}     & {77.1}       & {41.2}    & {53.8}  \\
\rowcolor{LightCyan}
SENet~\cite{Hu01}          & \tb{89.9} & \tb{92.0} & {\tb{67.3}} &  {\tb{79.4}} & {\tb{42.4}} & {\tb{57.5}}  \\
\bottomrule
\end{tabular}
\vspace{-5pt}
\caption{mAP comparison of Various \emph{BE} in our model. Training on SfM-120k.}
\label{tab:senet}
\end{table}
%------------------------------------------------------------------------------

\paragraph{ASPP \vs SKNet \vs SC}

Here we present the experimental comparison of ASPP~\cite{Chen2017RethinkingAC}, SKNet~\cite{sknet}, and our proposed \emph{selective context} (SC).
SC is a modified version of SKNet.
The modification is that instead of a simple \emph{element-wise sum} to initially fuse multiple Context information, it introduces a \emph{learnable parameter}~\eq{fuse} to fuse feature maps based on importance.
\autoref{tab:scm} presents these comparative results.
Our SC outperforms the other methods, reinforcing the efficacy of our approach in better embedding context information.
% \autoref{sec:1-stage}에서 제안한 \autoref{eq:sknet}의 ASPP, SKNet과 우리가 제안한 SCM에 대한 실험 비교이다.
% \autoref{tab:scm}은 이에 대한 실험 결과이다.
% 이 실험에서 우리의 SCM이 더 좋은 결과를 보인다.
% 이는 우리가 제안한 SCM이 Context 정보를 더 잘 embedding한다는 점을 보여준다고 해석할 수 있다.

%------------------------------------------------------------------------------
\begin{table}[t]
\centering
\scriptsize
%\tiny
\setlength{\tabcolsep}{6.0pt}
\begin{tabular}{l*{7}{c}} \toprule
\mr{2}{\Th{Method}} & \mr{2}{\Th{Oxf5k}} & \mr{2}{\Th{Par6k}} & \mc{2}{\Th{Medium}} & \mc{2}{\Th{Hard}} \\ \cmidrule(l){4-7}
 & & &  \rox & \rpa & \rox & \rpa \\ \midrule
ASPP~\cite{Chen2017RethinkingAC}  & \tb{90.3}   & 92.2    &  \tb{67.9} & 78.2 & 41.6 & 55.8\\
SKNet~\cite{sknet} & 89.3  & \tb{92.4} & {67.4} & 78.4 & 42.3 & 55.5 \\
\rowcolor{LightCyan}
SC (Ours) & {89.9} & {92.0} & {67.3} &  {\tb{79.4}}& {\tb{42.4}} & {\tb{57.5}}\\ \bottomrule
\end{tabular}
\vspace{-5pt}
\caption{mAP comparison of \emph{ASPP \vs SKNet \vs SC } in our model. Training on SfM-120k. SC: selective context}
\label{tab:scm}
\end{table}
%------------------------------------------------------------------------------

\paragraph{Sum (baseline) \vs learnable fusion}

We introduce learnable parameters~\eq{fuse} to fuse multiple feature maps, as described by SC and AL.
\autoref{tab:learnablefusing} shows the results of various ablation experiments when \emph{learnable fusing} and \emph{summing fusing} are applied together for SC and AL.
In this experiment, we evaluate four different ablation forms. The results indicate that three of these—SC, AL, and the combined SC+AL—perform better with learnable parameters than with simple summation.

% \autoref{sec:1-stage}에서 SCM과 ALM에 \autoref{eq:fuse-bifpn}를 이용하여 여러 feature map을 fusing할때, learnable parameters을 이용한다.
% \autoref{tab:learnablefusing}은 learnable-fusing과 Sum operation에 대한 비교실험이다.
% 이 실험에서 각각의 4가지 형태의 ablation 평가를 했는데, Sum operation (base) 만 적용했을때보다, learnable parameters를 사용했을때의 3가지 ablation(SCM, ALM, SCM+ALM)이 더 높았음을 보여주고 있다.

%------------------------------------------------------------------------------
\begin{table}[t]
\centering
\scriptsize
\setlength{\tabcolsep}{5.5pt}
\begin{tabular}{l*{9}{c}} \toprule
& \mr{2}{SC} & \mr{2}{AL} & \mr{2}{\Th{Oxf5k}} & \mr{2}{\Th{Par6k}} & \mc{2}{\Th{Medium}} & \mc{2}{\Th{Hard}} \\ \cmidrule(l){6-9}
 & & & &  & \rox & \rpa & \rox & \rpa  \\ \midrule
&     &      &   87.1    & 90.6       & 63.9       & 77.3     & 36.7      & 53.9 \\
& \ch &      &   87.6    & 90.8       & 64.7       & 77.8      & 37.9      & 54.8 \\
&     &   \ch   &   89.7    & 92.0       & 66.8       &   \tb{79.4}    & 41.8      & \tb{57.5} \\
& \ch & \ch  & \tb{89.9} & \tb{92.0} & \tb{67.3} & \tb{79.4} & \tb{42.4} & \tb{57.5} \\
\bottomrule
\end{tabular}
\vspace{-8pt}
\caption{mAP comparison of \emph{learnable-fusing \vs sum fusing. \ch is learnnable-fusing}. Training on SfM-120k. SC: selective context; AL: attentional localization.}
\label{tab:learnablefusing}
\end{table}
%------------------------------------------------------------------------------

\paragraph{Attention based Pooling \vs Mask based Pooling}

%------------------------------------------------------------------------------
\begin{table}[t]
\centering
\scriptsize
%\tiny
\setlength{\tabcolsep}{3.0pt}
\begin{tabular}{l*{7}{c}} \toprule
\mr{2}{\Th{Backbone}} & \mr{2}{\Th{Oxf5k}} & \mr{2}{\Th{Par6k}} & \mc{2}{\Th{Medium}} & \mc{2}{\Th{Hard}} \\ \cmidrule(l){4-7}
 & & &  \rox & \rpa & \rox & \rpa \\ \midrule
Attention based Pooling           & 89.8      & \tb{92.3} & 67.2      &  \tb{79.4}    & 41.8      & 56.5  \\
\rowcolor{LightCyan}
Mask based Pooling (Ours) & \tb{89.9} & {92.0}    & \tb{67.3}&  \tb{79.4}& \tb{42.4} & \tb{57.6}\\ \bottomrule
\end{tabular}
\vspace{-5pt}
\caption{mAP comparison of pr-trained model about \emph{Attention based Pooling \vs Mask based Pooling}. Training on SfM-120k.}
\label{tab:pooling}
\end{table}
%------------------------------------------------------------------------------

Spatial attention map \eq{attn} in \autoref{sec:1-stage} may be interpreted in a variety of ways. In our case, by using it to remove the background, it creates a focused feature on the Object.
Our research, CiDeR, can be called \emph{Mask based Pooling}. In the application of $1 \times 1$ convolution in \eq{attn}, it is equal to the weight vector of the dot product of each patch feature, which can be seen as CLS embedding. Therefore, it is equivalent to $QK^\top$ in the self attention mechanism, where Q is CLS and K is the patches. So, if we apply softmax instead of ``softplus followed by $\ell_1$ normalization'' in \eq{attn}, we have $A = softmax(QK^\top)$.
Next, if we directly multiply A by F, we get $softmax(QK^\top)V \in \real^{w \times h \times D}$, which is equivalent to self attention.
The feature generated here can be applied to a pooling algorithm like GeM, and we call  \emph{Attention based Pooling}~\cite{pmlr-v139-radford21a, touvron2021augmenting, psomas2023simpool}.
\autoref{tab:pooling} is a comparison experiment for these two poolings.
From these results, we can see that mask based pooling performs slightly better than attention based pooling.

%------------------------------------------------------------------------------

\paragraph{Feature Dimension}

After applying spatial pooling like GeM, we apply FC to generate the final feature. The feature dimension is determined by the hyperparameters. \autoref{tab:dimension} presents these experimental results. Interestingly, a feature dimension of 2048 emerges as optimal, with larger dimensions not necessarily offering any performance improvements.
% 우리의 모델에서 global represenataion은 \autoref{eq:Bottleneck}에 의해 표현된다.
% 이 수식의 마지막 \tb{FC}의 dimension을 의미한다.
% \autoref{tab:dimension}은 이에 대한 결과를 보여준다.
% 이 결과에서 dimension이 2048일때 가장 좋았고, 이보다 더 큰 dimension이 반드시 더 나은 성능을 보여주지는 않는다.

%------------------------------------------------------------------------------
\begin{table}[t]
\centering
\scriptsize
%\tiny
\setlength{\tabcolsep}{8.0pt}
\begin{tabular}{l*{7}{c}} \toprule
\mr{2}{\Th{Dim}} & \mr{2}{\Th{Oxf5k}} & \mr{2}{\Th{Par6k}} & \mc{2}{\Th{Medium}} & \mc{2}{\Th{Hard}} \\ \cmidrule(l){4-7}
 & & &  \rox & \rpa & \rox & \rpa \\ \midrule
4096 & 87.8 & 90.2 & 64.8 &  76.8 & 38.1 & 52.8 \\
3097 & 89.8 & 90.5 & \tb{67.4} &  76.9 & \tb{42.5} & 53.0 \\
\rowcolor{LightCyan}
2048 & \tb{89.9} & \tb{92.0} & {67.3} &  {\tb{79.4}}& {{42.4}} & {\tb{57.5}}\\
1024 & 88.9  & 91.2  & 65.7 &  76.7 & 40.1 & 52.0 \\
512  & 85.3  & 89.2  & 61.9 &  74.4 & 36.5 & 48.9 \\
\bottomrule
\end{tabular}
\vspace{-5pt}
\caption{mAP comparison of different \emph{features dimension} in our model. Training on SfM-120k.}
\label{tab:dimension}
\end{table}
%------------------------------------------------------------------------------

\paragraph{Multi-resolution}

For the final feature during inference, we employ a multi-resolution representation method that uses various image scales (0.4, 0.5, 0.7, 1.0, 1.4) for both the query and the database images. Features are extracted at each scale and then averaged to constitute the final feature. ~\autoref{tab:QE} provides a comparative analysis of results, both with and without the application of multi-resolution representation for queries and databases. We identify optimal queries and databases for \roxf and \rpar ~\cite{RITAC18}, particularly when multi-resolution is applied.

% 우리는 inference시 최종 feature에 대해 multi-resolution representation 방법을 사용한다.
% 이 방법은 query와 database에 대해 다양한 image scale (0.4, 0.5, 0.7, 1.0, 1.4) 로 구성하고, 각각 feature를 추출한다.
% 각 스케일의 모든 feature를 평균화하여 최종 feature로 구성한다.
% ~\autoref{tab:QE}는 query와 database에 대해 multi-resolution representation을 적용했을때와 적용하지 않았을때의 비교실험에 대한 결과를 보여준다.
% 우리는 \roxf  와  \rpar ~\cite{RITAC18}에 더 좋은 query와 database와 multi-resolution 일 경우 선택하였다.

%------------------------------------------------------------------------------
\begin{table}
\centering
\scriptsize
\setlength{\tabcolsep}{4.0pt}
\begin{tabular}{l*{7}{c}} \toprule
\mr{2}{\Th{Query}} & \mr{2}{\Th{Database}} & \mr{2}{\Th{Oxf5k}} & \mr{2}{\Th{Par6k}} & \mc{2}{\Th{$\cR$Medium}} & \mc{2}{\Th{$\cR$Hard}} \\ \cmidrule(l){5-8}
 & & & & \rox & \rpa & \rox & \rpa \\ \midrule
Single & Single &  90.5 & 91.5 & 67.0 & 77.4 & 40.3 & 55.0 \\
Multi & Single &  \tb{92.6} & \tb{92.9} & \tb{68.4} & {79.2} & 41.2 & 56.5 \\
Single & Multi & 87.1 & 90.4 & 64.8 & 77.5 & 39.1 & 55.9 \\
\rowcolor{LightCyan}
Multi & Multi & {89.9} & {92.0} & {67.3} &  {\tb{79.4}}& {\tb{42.4}} & {\tb{57.5}}\\  \bottomrule
\end{tabular}
\vspace{-6pt}
\caption{mAP comparison using \emph{Multiresolution} representation (Multi) or not (Single) on query or database. Training on SfM-120k.}
\label{tab:QE}
\end{table}
%------------------------------------------------------------------------------

\paragraph{ImageNet pre-trained models}

Various research groups have released ImageNet~\cite{Russakovsky01} pre-trained models for major image classification tasks. In general, ResNet101 employs a pre-trained model sourced from Torchvision~\cite{torchvision}. Recent works~\cite{yang2021dolg, cvnet} have also leveraged pre-trained models released by Facebook\footnote{\url{https://github.com/facebookresearch/pycls}}. In our experiments, as outlined in \autoref{tab:backbone}, we find that the Torchvision model outperforms its counterparts.
% 다양한 연구 단체에서 주요 이미지 분류에 대한 Pre-trained Model를 공개해왔다.
% 일반적으로 ResNet101은 Torchvision~\cite{torchvision}의 Pre-trained model를 사용한다.
% 최근 몇몇 연구~\cite{yang2021dolg, cvnet}는 Facebook\footnote{https://github.com/facebookresearch/pycls}에서 공개된 Pre-trained model를 사용한 경우가 있다.
% \autoref{tab:backbone}은 이러한 다양한 Pre-trained model에 대해 우리의 방법을 비교한다.
% 이 실험에서 Torchvision 모델을 사용할때 더 좋은 성능을 보였다.

%------------------------------------------------------------------------------
\begin{table}[t]
\centering
\scriptsize
%\tiny
\setlength{\tabcolsep}{6.0pt}
\begin{tabular}{l*{7}{c}} \toprule
\mr{2}{\Th{Backbone}} & \mr{2}{\Th{Oxf5k}} & \mr{2}{\Th{Par6k}} & \mc{2}{\Th{Medium}} & \mc{2}{\Th{Hard}} \\ \cmidrule(l){4-7}
 & & &  \rox & \rpa & \rox & \rpa \\ \midrule
Facebook           & 88.2      & \tb{92.7} & 65.3      &  78.8    & 38.6      & 56.5  \\
\rowcolor{LightCyan}
TorchVision & \tb{89.9} & {92.0}    & \tb{67.3}&  \tb{79.4}& \tb{42.4} & \tb{57.5}\\ \bottomrule
\end{tabular}
\vspace{-5pt}
\caption{mAP comparison of pr-trained model about \emph{Torchvision \vs Facebook}. Training on SfM-120k.}
\label{tab:backbone}
\end{table}
%------------------------------------------------------------------------------

\paragraph{Warm-Up}

To enhance model performance, we implement a warm-up phase~\cite{He2018BagOT} during training, consisting of three warming-up epochs. The outcomes, summarized in ~\autoref{tab:Warmup}, reveal a performance uptick when incorporating the warm-up approach.
% 우리는 성능을 향상시키기 위해 warm-up~\cite{He2018BagOT}을 적용한다.
% 학습시 우리는 3 warming-up epochs을 적용하여 실험에 적용한다.
% ~\autoref{tab:Warmup}은 이에 대한 실험 결과이다.
% 이 결과에서, warm-up을 적용할때 결과가 더 좋았음을 보여준다.

%------------------------------------------------------------------------------
\begin{table}[t]
\centering
\scriptsize
%\tiny
\setlength{\tabcolsep}{5.6pt}
\begin{tabular}{l*{7}{c}} \toprule
\mr{2}{\Th{Warm-up}} & \mr{2}{\Th{Oxf5k}} & \mr{2}{\Th{Par6k}} & \mc{2}{\Th{Medium}} & \mc{2}{\Th{Hard}} \\ \cmidrule(l){4-7}
 & & &  \rox & \rpa & \rox & \rpa \\ \midrule
w/o Warm-up            & \tb{89.9}  & \tb{92.0} & 66.7      &  78.9      & 41.5      & 56.7  \\
\rowcolor{LightCyan}
w/ Warm-up        & \tb{89.9}  & \tb{92.0} & \tb{67.3} &  \tb{79.4} & \tb{42.4} & \tb{57.5}\\ \bottomrule
\end{tabular}
\vspace{-5pt}
\caption{mAP comparison of \emph{Warm-Up} (with \vs without) in our model. Training on SfM-120k.}
\label{tab:Warmup}
\end{table}
%------------------------------------------------------------------------------

\paragraph{Whitening}

We utilize the supervised whitening method pioneered by Radenović~\etal~\cite{Radenovic01}, which is frequently employed in similar research to enhance model efficacy. ~\autoref{tab:whitening} showcases the performance gains realized through the application of whitening techniques.
% Radenović~\etal~\cite{Radenovic01}에서 적용했던 supervised whitening 방법을 이용한다.
% 이 방법은 성능향상의 하나의 방법으로써 많은 유사한 연구에서 적용되고있다.
% ~\autoref{tab:whitening}은 whitening을 적용한 결과를 보여준다.
% 이 결과에서, whitening을 적용했을때, 성능이 향상된것을 볼 수 있다.

%------------------------------------------------------------------------------
\begin{table}[t]
\centering
\scriptsize
%\tiny
\setlength{\tabcolsep}{5.3pt}
\begin{tabular}{l*{7}{c}} \toprule
\mr{2}{\Th{whitening}} & \mr{2}{\Th{Oxf5k}} & \mr{2}{\Th{Par6k}} & \mc{2}{\Th{Medium}} & \mc{2}{\Th{Hard}} \\ \cmidrule(l){4-7}
 & & &  \rox & \rpa & \rox & \rpa \\ \midrule
w/o Whitening   & 85.8      & 90.7      & 60.5      &  77.0    & 31.7      & 54.2  \\
\rowcolor{LightCyan}
w/ Whitening   & \tb{89.9} & \tb{92.0}     & \tb{67.3} & \tb{79.4}& \tb{42.4} & \tb{57.5}\\ \bottomrule
\end{tabular}
\vspace{-5pt}
\caption{mAP comparison of \emph{Whitening} (with \vs without) in our model. Training on SfM-120k.}
\label{tab:whitening}
\end{table}
%------------------------------------------------------------------------------

\paragraph{Fixed-size \vs Group-size sampling}

%------------------------------------------------------------------------------
\begin{table}
\centering
\scriptsize
\setlength{\tabcolsep}{4.2pt}
\begin{tabular}{l*{6}{c}} \toprule
\mr{2}{\Th{Method}} & \mr{2}{\Th{Oxf5k}} & \mr{2}{\Th{Par6k}} & \mc{2}{\Th{$\cR$Medium}} & \mc{2}{\Th{$\cR$Hard}} \\ \cmidrule(l){4-7}
 & & & \rox & \rpa & \rox & \rpa \\ \midrule
Fixed-size (224 × 224) & 69.0 & 86.0 & 42.2 & 69.5 & 15.8 & 45.0\\
\rowcolor{LightCyan}
Group-size (Ours) & \tb{89.9}  & \tb{92.0} & \tb{67.3} &  \tb{79.4} & \tb{42.4} & \tb{57.5} \\
\bottomrule
\end{tabular}
\vspace{-6pt}
\caption{mAP comparison between \emph{Fixed-size ($224 \times 224$) \vs Group-size sampling} methods. Training on SfM-120k.}
\label{tab:groupsize}
\end{table}
%------------------------------------------------------------------------------

Several previous studies suggest organizing training batches based on image size for efficient learning.
Methods such as DIR~\cite{Gordo01}, DELF~\cite{delf}, MobileViT~\cite{mehta2021mobilevit}, and Yokoo~\etal\cite{Yokoo01} opt for variable image sizes rather than adhering to a single, fixed dimension.
Our approach employs group-size sampling~\cite{Yokoo01, SCH01, dtop}, where we construct image batches with similar aspect ratios.
\autoref{tab:groupsize} compares the results between fixed-size (224 × 224) and group-size sampling.
Our findings underscore the effectiveness of using dynamic input sizes to preserve the aspect ratio.

% 이전 다양한 연구들은 효율적인 훈련을 위해 이미지 크기에 따라 배치를 구성하는 방법을 제안한다.
% 예를 들어, DIR~\cite{Gordo01}, DELF~\cite{delf}, MobileViT~\cite{mehta2021mobilevit}, 그리고 Yokoo~\etal\cite{Yokoo01}는 단일 고정 크기 아닌 다양한 크기를 적용한다.
% \autoref{sec:Implementation}에 언급했듯이, 이 방법은 이미지의 aspect ratio가 유사한 이미지로 배치를 구성하고, aspect ratio가 유사한 데이터를 샘플링하여 학습하도록 한다(group-size sampling~\cite{Yokoo01, SCH01, dtop}).
% % 이미지를 해당 이미지의 종횡비와 유사한 크기로 샘플링하여 학습하도록 한다(group-size sampling~\cite{Yokoo01, SCH01, dtop}).
% \autoref{tab:groupsize}은 고정 크기 (224 × 224)와 그룹 크기 샘플링을 비교한 결과를 보여준다.
% 우리는 동적인 입력 크기를 사용하여 aspect ratio를 유지하는 것이 훨씬 효과적임을 관찰하였다.
